# Supplementary material for: AMR Parsing via Graph-Sequence Iterative Inference
Source: arXiv:2004.05572 source file (2020-04-29)
Supplement: Supplementary file 1 [file appendix.pdf]

# Appendix Section for AMR Parsing via Graph-Sequence Iterative Inference

Anonymous ACL submission

## A Hyper-parameter Settings

Table 1 lists the hyper-parameters used in our full models. Char-level CNNs and Transformer layers in the sentence encoder and the graph encoder share the same hyper-parameter settings. The BERT model (Devlin et al., 2019) we used is the Huggingface's implementation (Wolf et al., 2019) (bert-base-cased). To mitigate overfitting, we apply dropout (Srivastava et al., 2014) with the drop rate 0.2 between different layers. We randomly mask (replacing inputs with a special UNK token) the input lemmas, POS tags, and NER tags with a rate of 0.33. Parameter optimization is performed with the ADAM optimizer (Kingma and Ba, 2014) with $\beta_1 = 0.9$ and $\beta_2 = 0.999$. The learning rate schedule is similar to that in Vaswani et al. (2017), with warm-up steps being set to 2K. We use early stopping on the development set for choosing the best model. Our code is attached with this submission and will be released upon acceptance.

| | |
|---|---|
| **Embeddings** | |
| lemma | 300 |
| POS tag | 32 |
| NER tag | 16 |
| concept | 300 |
| char | 32 |
| **Char-level CNN** | |
| #filters | 256 |
| ngram filter size | [3] |
| output size | 128 |
| **Sentence Encoder** | |
| #transformer layers | 4 |
| **Graph Encoder** | |
| #transformer layers | 2 |
| **Transformer Layer** | |
| #heads | 8 |
| hidden size | 512 |
| feed-forward hidden size | 1024 |
| **Concept Solver** | |
| feed-forward hidden size | 1024 |
| **Relation Solver** | |
| #heads | 8 |
| feed-forward hidden size | 1024 |
| **Deep biaffine classifier** | |
| hidden size | 100 |

Table 1: Hyper-parameters settings.

## B AMR Pre- and Post-processing

We follow the exactly same pre- and post-processing steps of those of Zhang et al. (2019a,b) for graph re-categorization. In preprocessing, we anonymize entities, remove wiki links and polarity attributes, and convert the resultant AMR graphs into a compact format by compressing certain subgraphs. In post-processing, we recover the original AMR format from the compact format, restore Wikipedia links using the DBpedia Spotlight API (Daiber et al., 2013), add polarity attributes based on rules observed from the training data. More details can be found in Zhang et al. (2019a).

## References

Joachim Daiber, Max Jakob, Chris Hokamp, and Pablo N Mendes. 2013. Improving efficiency and accuracy in multilingual entity extraction. In *Proceedings of the 9th International Conference on Semantic Systems*, pages 121–124.

Jacob Devlin, Ming-Wei Chang, Kenton Lee, and Kristina Toutanova. 2019. BERT: Pre-training of deep bidirectional transformers for language understanding. In *Proceedings of the 2019 Conference of the North American Chapter of the Association for Computational Linguistics: Human Language Technologies, Volume 1 (Long and Short Papers)*, pages 4171–4186.

Diederik P Kingma and Jimmy Ba. 2014. Adam: A

method for stochastic optimization. *arXiv preprint arXiv:1412.6980*.

Nitish Srivastava, Geoffrey Hinton, Alex Krizhevsky, Ilya Sutskever, and Ruslan Salakhutdinov. 2014. Dropout: a simple way to prevent neural networks from overfitting. *The Journal of Machine Learning Research*, 15(1):1929–1958.

Ashish Vaswani, Noam Shazeer, Niki Parmar, Jakob Uszkoreit, Llion Jones, Aidan N Gomez, Łukasz Kaiser, and Illia Polosukhin. 2017. Attention is all you need. In *Advances in neural information processing systems*, pages 5998–6008.

Thomas Wolf, Lysandre Debut, Victor Sanh, Julien Chaumond, Clement Delangue, Anthony Moi, Pierric Cistac, Tim Rault, R'emi Louf, Morgan Funtowicz, and Jamie Brew. 2019. Huggingface's transformers: State-of-the-art natural language processing. *ArXiv*, abs/1910.03771.

Sheng Zhang, Xutai Ma, Kevin Duh, and Benjamin Van Durme. 2019a. AMR parsing as sequence-to-graph transduction. In *Proceedings of the 57th Annual Meeting of the Association for Computational Linguistics*, pages 80–94.

Sheng Zhang, Xutai Ma, Kevin Duh, and Benjamin Van Durme. 2019b. Broad-coverage semantic parsing as transduction. In *Proceedings of the 2019 Conference on Empirical Methods in Natural Language Processing and the 9th International Joint Conference on Natural Language Processing (EMNLP-IJCNLP)*, pages 3784–3796.
